# Supplementary material for: Tests of light-lepton universality in angular asymmetries of $B^0 \to D^{*-} \ell \nu$ decays
Source: arXiv:2308.02023 source file (2023-11-02)
Supplement: Supplementary file 1 [file supplemental_material.tex]

In Fig.~\ref{fig:equivalence}, we illustrate the equivalence between the definitions of \sthree, \sfive, \sseven, and \snine{} found in Ref.~\cite{bhattacharya} and the one-dimensional reinterpretation described in the text. In Table~\ref{tab:results_sm}, we show the results for all $\mathcal{A}$ and \deltaA{} observables in the three $w$ ranges, with uncertainties classified by source in Table~\ref{tab:systematics_sm}. We show the statistical and systematic covariance matrices in Figs.~\ref{fig:cov_stats} and \ref{fig:cov_syst}, respectively. 

% Without this, latex insists on putting figs above the section header. Using flafter does the same thing as this. 
\clearpage

\begin{figure}
  \centering
  \begin{subfigure}[b]{\linewidth}
    \includegraphics[scale=.8]{figures/tikz/s3.pdf}
    \tikz[scale=0.8]{
      \draw[draw=none] (0, -1) rectangle (0.2, 1.2) node [pos=.5] {\LARGE\(\equiv\)};
    }
    \includegraphics[scale=.8]{figures/tikz/s3-transformed.pdf}
    \captionsetup{justification=centering}
    \caption{\sthree\label{fig:s3}}
  \end{subfigure}
  \begin{subfigure}[b]{\linewidth}
    \includegraphics[scale=.8]{figures/tikz/s5.pdf}
    \tikz[scale=0.8]{
      \draw[draw=none] (0, -2) rectangle (0.2, 1.2) node [pos=.5] {\LARGE\(\equiv\)};
    }
    \includegraphics[scale=.8]{figures/tikz/s5-transformed.pdf}
    \captionsetup{justification=centering}
    \caption{\sfive\label{fig:s5}}
  \end{subfigure}
  \begin{subfigure}[b]{\linewidth}
    \includegraphics[scale=.8]{figures/tikz/s7.pdf}
    \tikz[scale=0.8]{
      \draw[draw=none] (0, -2) rectangle (0.2, 1.2) node [pos=.5] {\LARGE\(\equiv\)};
    }
    \includegraphics[scale=.8]{figures/tikz/s7-transformed.pdf}
    \captionsetup{justification=centering}
    \caption{\sseven\label{fig:s7}}
  \end{subfigure}
  \begin{subfigure}[b]{\linewidth}
    \includegraphics[scale=.8]{figures/tikz/s9.pdf}
    \tikz[scale=0.8]{
      \draw[draw=none] (0, -1) rectangle (0.2, 1.2) node [pos=.5] {\LARGE\(\equiv\)};
    }
    \includegraphics[scale=.8]{figures/tikz/s9-transformed.pdf}
    \captionsetup{justification=centering}
    \caption{\snine\label{fig:s9}}
  \end{subfigure}
  \captionsetup{justification=centering}
  %\caption{An illustration of the equivalence between the asymmetry categories of Ref.~\cite{bhattacharya} and our one-dimensionalized categories.}
  \caption{An illustration of the equivalence between the two-dimensional asymmetry categories of Ref.~\cite{bhattacharya} and our one-dimensional categories. All asymmetry variables are defined as normalized differences between yields of + (blue) and - (yellow) regions of their respective angular variable(s).}
  \label{fig:equivalence}
\end{figure}

\begin{table}
\centering
\caption{: Full results and total uncertainties from all angular observables along with the standard model expectations.}
\label{tab:results_sm}
\begin{tabular}{llrc}
\toprule
                     Obs. &             $w$ bin &       Measurement &    SM \\
\midrule
      $A_{\mathrm{FB}}^e$ &    $w_\mathrm{low}$ &   $0.149\pm0.045$ &   $\phantom{-}0.272\pm0.005$ \\
                          &   $w_\mathrm{high}$ &   $0.213\pm0.051$ &   $\phantom{-}0.209\pm0.003$ \\
                          &  $w_\mathrm{incl.}$ &   $0.183\pm0.033$ &   $\phantom{-}0.244\pm0.004$ \\
    $A_{\mathrm{FB}}^\mu$ &    $w_\mathrm{low}$ &    $0.248\pm0.040$ &  $\phantom{-}0.271\pm0.005$ \\
                          &   $w_\mathrm{high}$ &   $0.045\pm0.051$ &   $\phantom{-}0.198\pm0.003$ \\
                          &  $w_\mathrm{incl.}$ &   $0.158\pm0.032$ &   $\phantom{-}0.239\pm0.004$ \\
 $\Delta A_{\mathrm{FB}}$ &    $w_\mathrm{low}$ &    $0.099\pm0.060$ &  $\phantom{l000000}(-1.04\pm0.02)\times 10^{-3}$ \\
                          &   $w_\mathrm{high}$ &  $-0.168\pm0.073$ &   $\phantom{l00000}(-11.33\pm0.09)\times 10^{-3}$ \\
                          &  $w_\mathrm{incl.}$ &  $-0.024\pm0.046$ &   $\phantom{l000000}(-5.66\pm0.06)\times 10^{-3}$ \\
                  $S_3^e$ &    $w_\mathrm{low}$ &  $-0.133\pm0.053$ &   $-0.147\pm0.002$ \\
                          &   $w_\mathrm{high}$ &  $-0.016\pm0.053$ &   $-0.063\pm0.002$ \\
                          &  $w_\mathrm{incl.}$ &   $-0.080\pm0.037$ &  $-0.110\pm0.002$ \\
                $S_3^\mu$ &    $w_\mathrm{low}$ &  $-0.159\pm0.048$ &   $-0.147\pm0.002$ \\
                          &   $w_\mathrm{high}$ &  $-0.117\pm0.051$ &   $-0.063\pm0.002$ \\
                          &  $w_\mathrm{incl.}$ &  $-0.142\pm0.034$ &   $-0.110\pm0.002$ \\
             $\Delta S_3$ &    $w_\mathrm{low}$ &  $-0.026\pm0.072$ &   $\phantom{00000000}(0.279\pm0.002)\times 10^{-3}$ \\
                          &   $w_\mathrm{high}$ &  $-0.101\pm0.073$ &   $\phantom{00000000}(0.233\pm0.008)\times 10^{-3}$ \\
                          &  $w_\mathrm{incl.}$ &   $-0.062\pm0.050$ &  $\phantom{00000000}(0.176\pm0.005)\times 10^{-3}$ \\
                  $S_5^e$ &    $w_\mathrm{low}$ &   $0.166\pm0.054$ &   $\phantom{-}0.172\pm0.004$ \\
                          &   $w_\mathrm{high}$ &    $0.215\pm0.050$ &  $\phantom{-}0.221\pm0.004$ \\
                          &  $w_\mathrm{incl.}$ &    $0.190\pm0.036$ &  $\phantom{-}0.194\pm0.004$ \\
                $S_5^\mu$ &    $w_\mathrm{low}$ &   $0.146\pm0.049$ &   $\phantom{-}0.172\pm0.004$ \\
                          &   $w_\mathrm{high}$ &    $0.160\pm0.048$ &  $\phantom{-}0.222\pm0.004$ \\
                          &  $w_\mathrm{incl.}$ &   $0.155\pm0.034$ &   $\phantom{-}0.194\pm0.004$ \\
             $\Delta S_5$ &    $w_\mathrm{low}$ &  $-0.019\pm0.073$ &   $\phantom{00000000}(0.272\pm0.003)\times 10^{-3}$ \\
                          &   $w_\mathrm{high}$ &  $-0.055\pm0.069$ &   $\phantom{000000000}(1.07\pm0.04)\phantom{0}\times 10^{-3}$ \\
                          &  $w_\mathrm{incl.}$ &  $-0.035\pm0.049$ &   $\phantom{000000000}(0.49\pm0.02)\phantom{0}\times 10^{-3}$ \\
                  $S_7^e$ &    $w_\mathrm{low}$ &  $-0.088\pm0.053$ &     $\phantom{l000}0.0\pm0.0\phantom{00}$ \\
                          &   $w_\mathrm{high}$ &   $0.045\pm0.049$ &           $\phantom{-}0.0\pm0.0$ \\
                          &  $w_\mathrm{incl.}$ &  $-0.018\pm0.035$ &           $\phantom{-}0.0\pm0.0$ \\
                $S_7^\mu$ &    $w_\mathrm{low}$ &   $-0.060\pm0.047$ &           $\phantom{-}0.0\pm0.0$ \\
                          &   $w_\mathrm{high}$ &   $-0.020\pm0.047$ &           $\phantom{-}0.0\pm0.0$ \\
                          &  $w_\mathrm{incl.}$ &  $-0.043\pm0.033$ &           $\phantom{-}0.0\pm0.0$ \\
             $\Delta S_7$ &    $w_\mathrm{low}$ &   $0.028\pm0.071$ &           $\phantom{-}0.0\pm0.0$ \\
                          &   $w_\mathrm{high}$ &  $-0.066\pm0.069$ &           $\phantom{-}0.0\pm0.0$ \\
                          &  $w_\mathrm{incl.}$ &  $-0.026\pm0.049$ &           $\phantom{-}0.0\pm0.0$ \\
                  $S_9^e$ &    $w_\mathrm{low}$ &  $-0.035\pm0.054$ &           $\phantom{-}0.0\pm0.0$ \\
                          &   $w_\mathrm{high}$ &    $0.020\pm0.052$ &           $\phantom{-}0.0\pm0.0$ \\
                          &  $w_\mathrm{incl.}$ &  $-0.004\pm0.036$ &           $\phantom{-}0.0\pm0.0$ \\
                $S_9^\mu$ &    $w_\mathrm{low}$ &  $-0.003\pm0.048$ &           $\phantom{-}0.0\pm0.0$ \\
                          &   $w_\mathrm{high}$ &    $0.040\pm0.050$ &           $\phantom{-}0.0\pm0.0$ \\
                          &  $w_\mathrm{incl.}$ &   $0.016\pm0.034$ &           $\phantom{-}0.0\pm0.0$ \\
             $\Delta S_9$ &    $w_\mathrm{low}$ &   $0.032\pm0.071$ &           $\phantom{-}0.0\pm0.0$ \\
                          &   $w_\mathrm{high}$ &    $0.020\pm0.072$ &           $\phantom{-}0.0\pm0.0$ \\
                          &  $w_\mathrm{incl.}$ &     $0.020\pm0.050$ &           $\phantom{-}0.0\pm0.0$ \\
\bottomrule
\end{tabular}
\end{table}

\begin{table}
\centering
\caption{Summary of the experimental uncertainties for all angular observables (Obs.) classified by relevant source: sample size (Stat.), MC sample size (MC stat.), lepton ID (LID), and slow-pion efficiency ($\pi_{	\textrm{slow}}$).}
\label{tab:systematics_sm}
\begin{tabular}{llccccc}
\toprule
                     Obs. &             $w$ bin &  Total &  Stat. &  MC stat. &    LID &  $\pi_{\textrm{slow}}$ \\
\midrule
      $A_{\mathrm{FB}}^e$ &    $w_\mathrm{low}$ &  0.045 &  0.042 &     0.015 &  0.004 &                  0.001 \\
                          &   $w_\mathrm{high}$ &  0.051 &  0.048 &     0.017 &  0.004 &                  0.001 \\
                          &  $w_\mathrm{incl.}$ &  0.033 &  0.031 &     0.011 &  0.004 &                  0.001 \\
    $A_{\mathrm{FB}}^\mu$ &    $w_\mathrm{low}$ &  0.040 &  0.038 &     0.013 &  0.001 &                  0.001 \\
                          &   $w_\mathrm{high}$ &  0.051 &  0.048 &     0.016 &  0.002 &                  0.001 \\
                          &  $w_\mathrm{incl.}$ &  0.032 &  0.030 &     0.010 &  0.001 &                  0.001 \\
 $\Delta A_{\mathrm{FB}}$ &    $w_\mathrm{low}$ &  0.060 &  0.056 &     0.020 &  0.004 &                  0.001 \\
                          &   $w_\mathrm{high}$ &  0.073 &  0.068 &     0.024 &  0.004 &                  0.001 \\
                          &  $w_\mathrm{incl.}$ &  0.046 &  0.043 &     0.015 &  0.004 &                  0.001 \\
                  $S_3^e$ &    $w_\mathrm{low}$ &  0.053 &  0.050 &     0.018 &  $<0.001\phantom{0~~}$ &                  0.001 \\
                          &   $w_\mathrm{high}$ &  0.053 &  0.049 &     0.018 &  $<0.001\phantom{0~~}$ &                  $<0.001\phantom{0~~}$ \\
                          &  $w_\mathrm{incl.}$ &  0.037 &  0.034 &     0.012 &  $<0.001\phantom{0~~}$ &                  $<0.001\phantom{0~~}$ \\
                $S_3^\mu$ &    $w_\mathrm{low}$ &  0.048 &  0.045 &     0.016 &  0.001 &                  $<0.001\phantom{0~~}$ \\
                          &   $w_\mathrm{high}$ &  0.051 &  0.048 &     0.016 &  $<0.001\phantom{0~~}$ &                  $<0.001\phantom{0~~}$ \\
                          &  $w_\mathrm{incl.}$ &  0.034 &  0.032 &     0.011 &  0.001 &                  $<0.001\phantom{0~~}$ \\
             $\Delta S_3$ &    $w_\mathrm{low}$ &  0.072 &  0.068 &     0.024 &  0.001 &                  $<0.001\phantom{0~~}$ \\
                          &   $w_\mathrm{high}$ &  0.073 &  0.069 &     0.025 &  0.001 &                  $<0.001\phantom{0~~}$ \\
                          &  $w_\mathrm{incl.}$ &  0.050 &  0.047 &     0.017 &  0.001 &                  $<0.001\phantom{0~~}$ \\
                  $S_5^e$ &    $w_\mathrm{low}$ &  0.054 &  0.051 &     0.018 &  0.001 &                  $<0.001\phantom{0~~}$ \\
                          &   $w_\mathrm{high}$ &  0.050 &  0.047 &     0.017 &  0.001 &                  $<0.001\phantom{0~~}$ \\
                          &  $w_\mathrm{incl.}$ &  0.036 &  0.034 &     0.012 &  0.001 &                  $<0.001\phantom{0~~}$ \\
                $S_5^\mu$ &    $w_\mathrm{low}$ &  0.049 &  0.046 &     0.016 &  0.001 &                  $<0.001\phantom{0~~}$ \\
                          &   $w_\mathrm{high}$ &  0.048 &  0.045 &     0.016 &  $<0.001\phantom{0~~}$ &                  $<0.001\phantom{0~~}$ \\
                          &  $w_\mathrm{incl.}$ &  0.034 &  0.032 &     0.011 &  $<0.001\phantom{0~~}$ &                  $<0.001\phantom{0~~}$ \\
             $\Delta S_5$ &    $w_\mathrm{low}$ &  0.073 &  0.068 &     0.024 &  0.001 &                  $<0.001\phantom{0~~}$ \\
                          &   $w_\mathrm{high}$ &  0.069 &  0.065 &     0.023 &  0.001 &                  $<0.001\phantom{0~~}$ \\
                          &  $w_\mathrm{incl.}$ &  0.049 &  0.046 &     0.016 &  0.001 &                  $<0.001\phantom{0~~}$ \\
                  $S_7^e$ &    $w_\mathrm{low}$ &  0.053 &  0.050 &     0.018 &  0.001 &                  $<0.001\phantom{0~~}$ \\
                          &   $w_\mathrm{high}$ &  0.049 &  0.046 &     0.017 &  $<0.001\phantom{0~~}$ &                  $<0.001\phantom{0~~}$ \\
                          &  $w_\mathrm{incl.}$ &  0.035 &  0.033 &     0.012 &  $<0.001\phantom{0~~}$ &                  $<0.001\phantom{0~~}$ \\
                $S_7^\mu$ &    $w_\mathrm{low}$ &  0.047 &  0.045 &     0.015 &  $<0.001\phantom{0~~}$ &                  $<0.001\phantom{0~~}$ \\
                          &   $w_\mathrm{high}$ &  0.047 &  0.045 &     0.015 &  $<0.001\phantom{0~~}$ &                  $<0.001\phantom{0~~}$ \\
                          &  $w_\mathrm{incl.}$ &  0.033 &  0.031 &     0.011 &  $<0.001\phantom{0~~}$ &                  $<0.001\phantom{0~~}$ \\
             $\Delta S_7$ &    $w_\mathrm{low}$ &  0.071 &  0.067 &     0.023 &  0.001 &                  0.001 \\
                          &   $w_\mathrm{high}$ &  0.069 &  0.065 &     0.022 &  $<0.001\phantom{0~~}$ &                  $<0.001\phantom{0~~}$ \\
                          &  $w_\mathrm{incl.}$ &  0.049 &  0.046 &     0.016 &  $<0.001\phantom{0~~}$ &                  $<0.001\phantom{0~~}$ \\
                  $S_9^e$ &    $w_\mathrm{low}$ &  0.054 &  0.050 &     0.018 &  $<0.001\phantom{0~~}$ &                  $<0.001\phantom{0~~}$ \\
                          &   $w_\mathrm{high}$ &  0.052 &  0.049 &     0.018 &  $<0.001\phantom{0~~}$ &                  $<0.001\phantom{0~~}$ \\
                          &  $w_\mathrm{incl.}$ &  0.036 &  0.034 &     0.012 &  $<0.001\phantom{0~~}$ &                  $<0.001\phantom{0~~}$ \\
                $S_9^\mu$ &    $w_\mathrm{low}$ &  0.048 &  0.046 &     0.016 &  $<0.001\phantom{0~~}$ &                  $<0.001\phantom{0~~}$ \\
                          &   $w_\mathrm{high}$ &  0.050 &  0.047 &     0.016 &  $<0.001\phantom{0~~}$ &                  0.001 \\
                          &  $w_\mathrm{incl.}$ &  0.034 &  0.032 &     0.011 &  $<0.001\phantom{0~~}$ &                  $<0.001\phantom{0~~}$ \\
             $\Delta S_9$ &    $w_\mathrm{low}$ &  0.071 &  0.067 &     0.024 &  $<0.001\phantom{0~~}$ &                  $<0.001\phantom{0~~}$ \\
                          &   $w_\mathrm{high}$ &  0.072 &  0.068 &     0.024 &  0.001 &                  0.001 \\
                          &  $w_\mathrm{incl.}$ &  0.050 &  0.047 &     0.017 &  $<0.001\phantom{0~~}$ &                  $<0.001\phantom{0~~}$ \\
\bottomrule
\end{tabular}
\end{table}

\begin{figure*}[b]
  \centering
    \includegraphics[width=\textwidth]{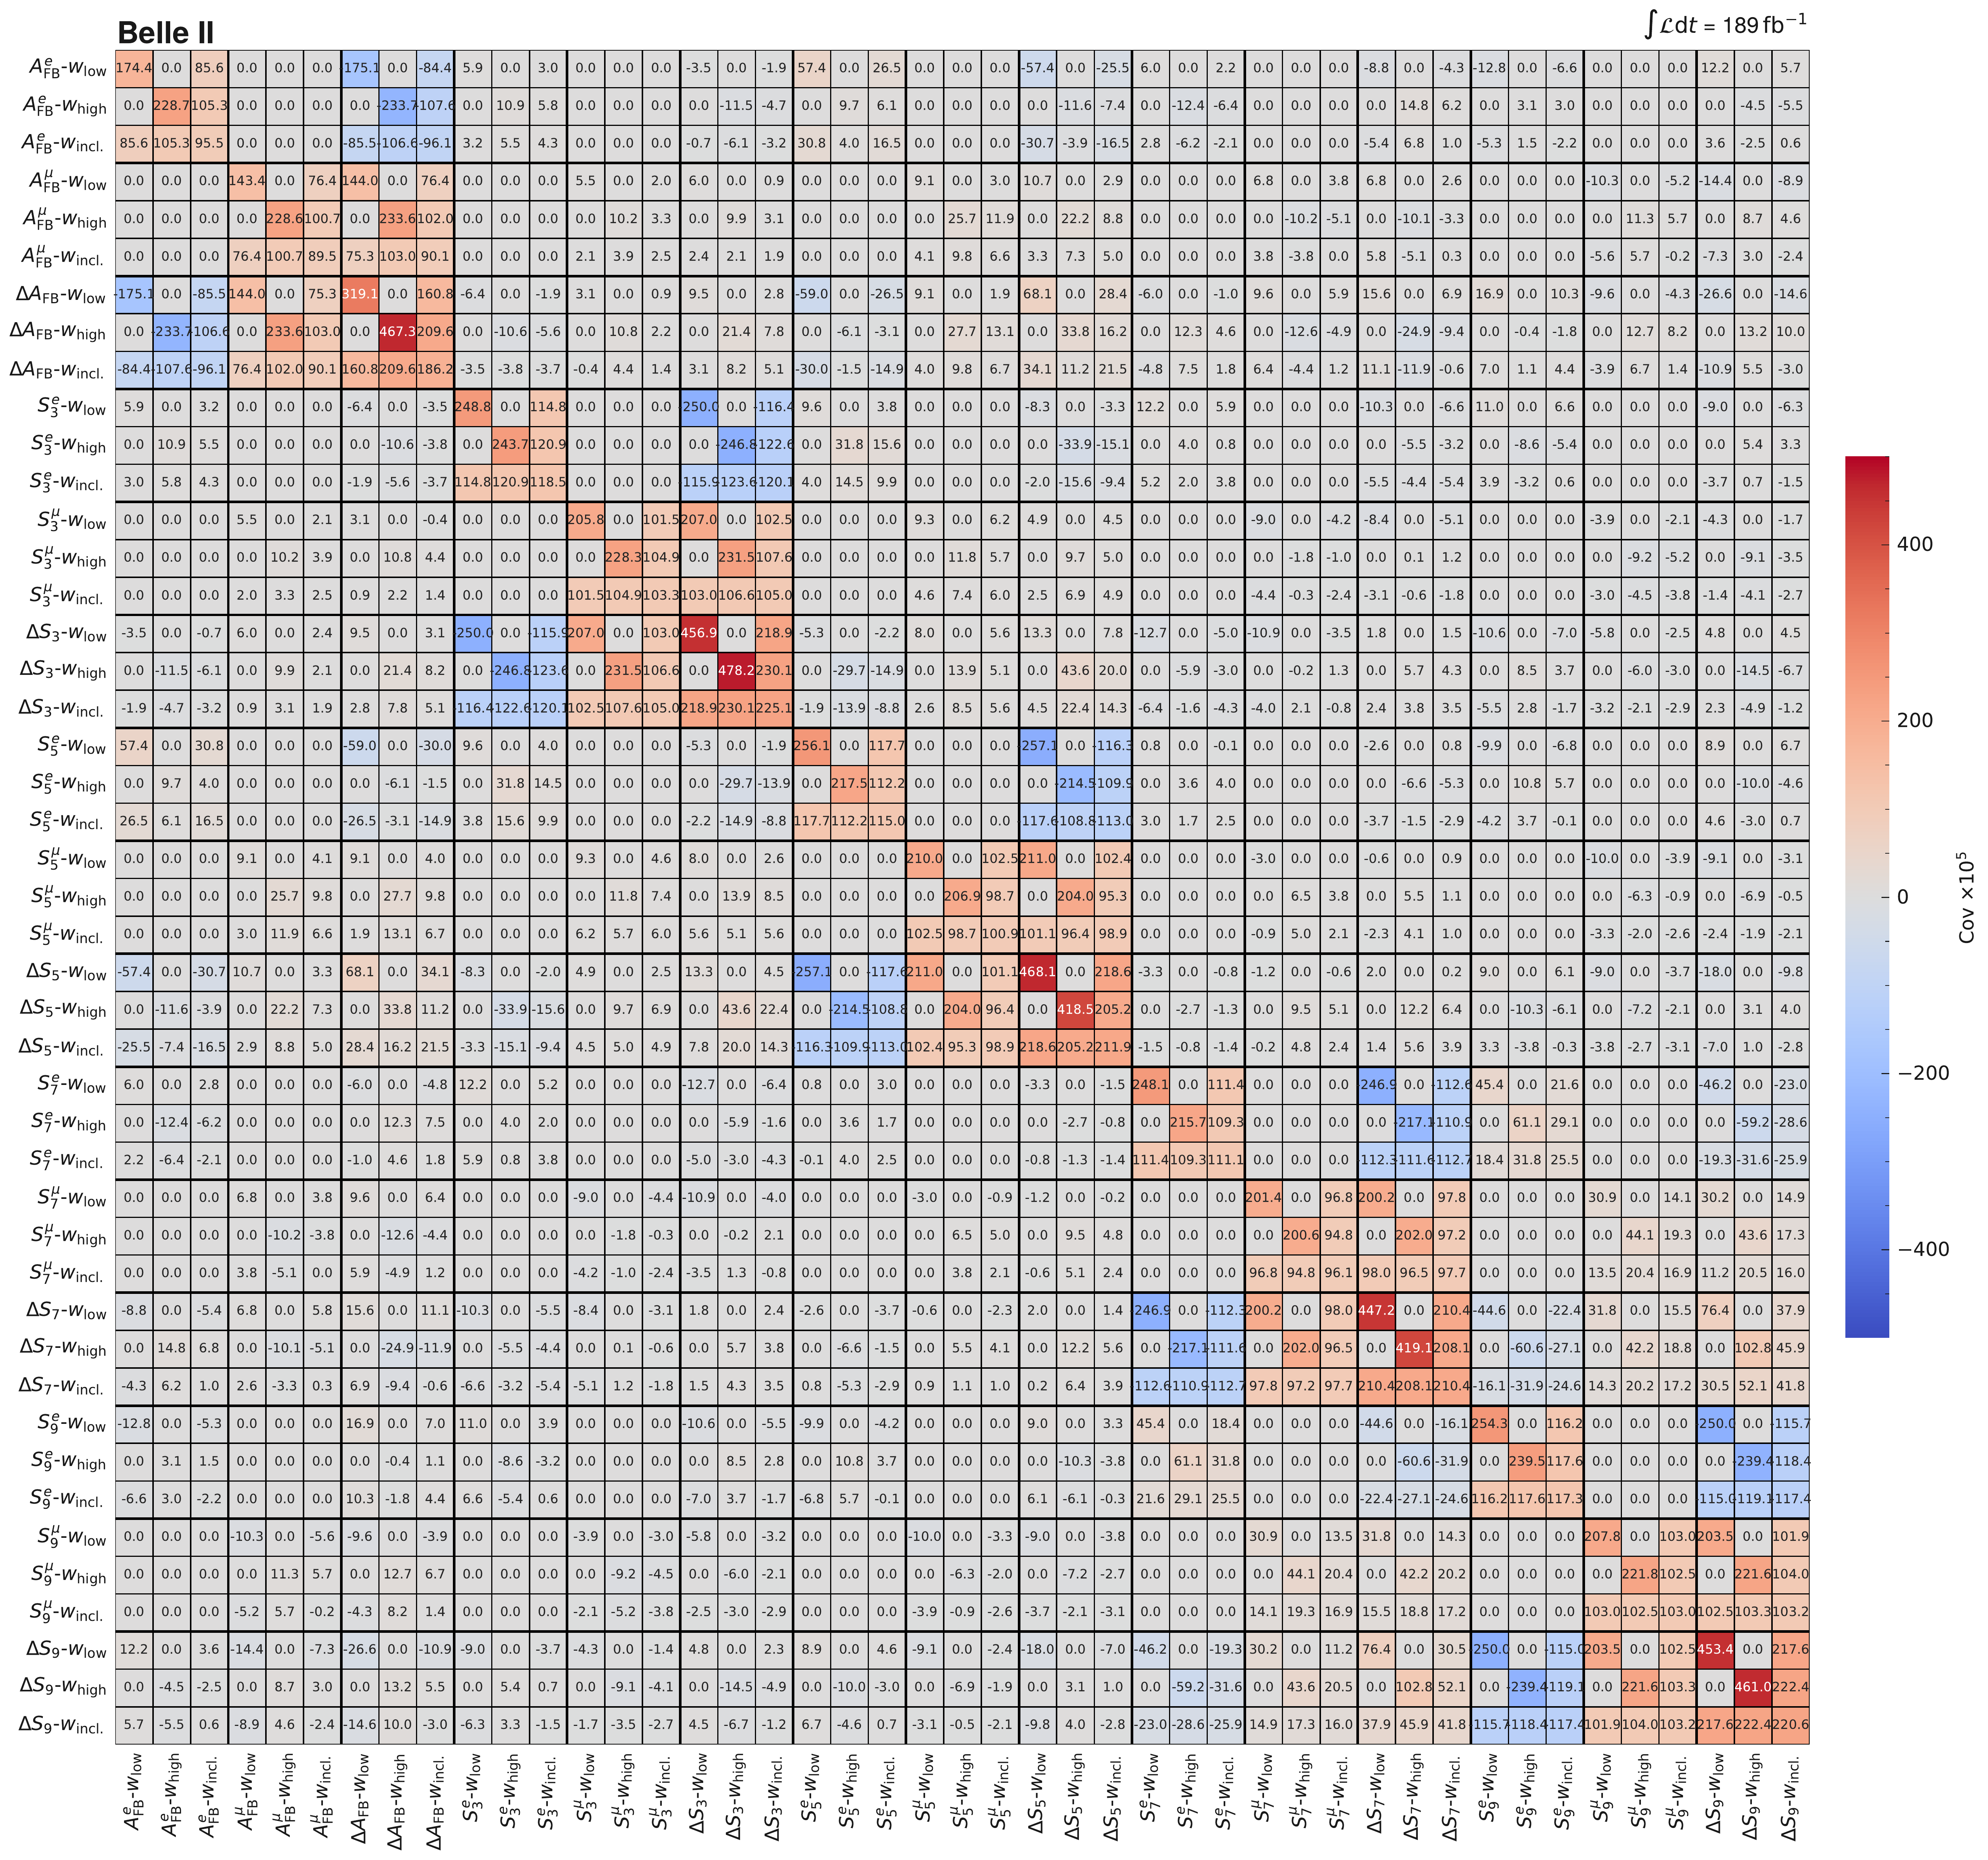}

  \caption{Statistical covariance matrix determined by sampling experimental data with replacement.}
  \label{fig:cov_stats}
\end{figure*}

\begin{figure*}
  \centering
    \includegraphics[width=\textwidth]{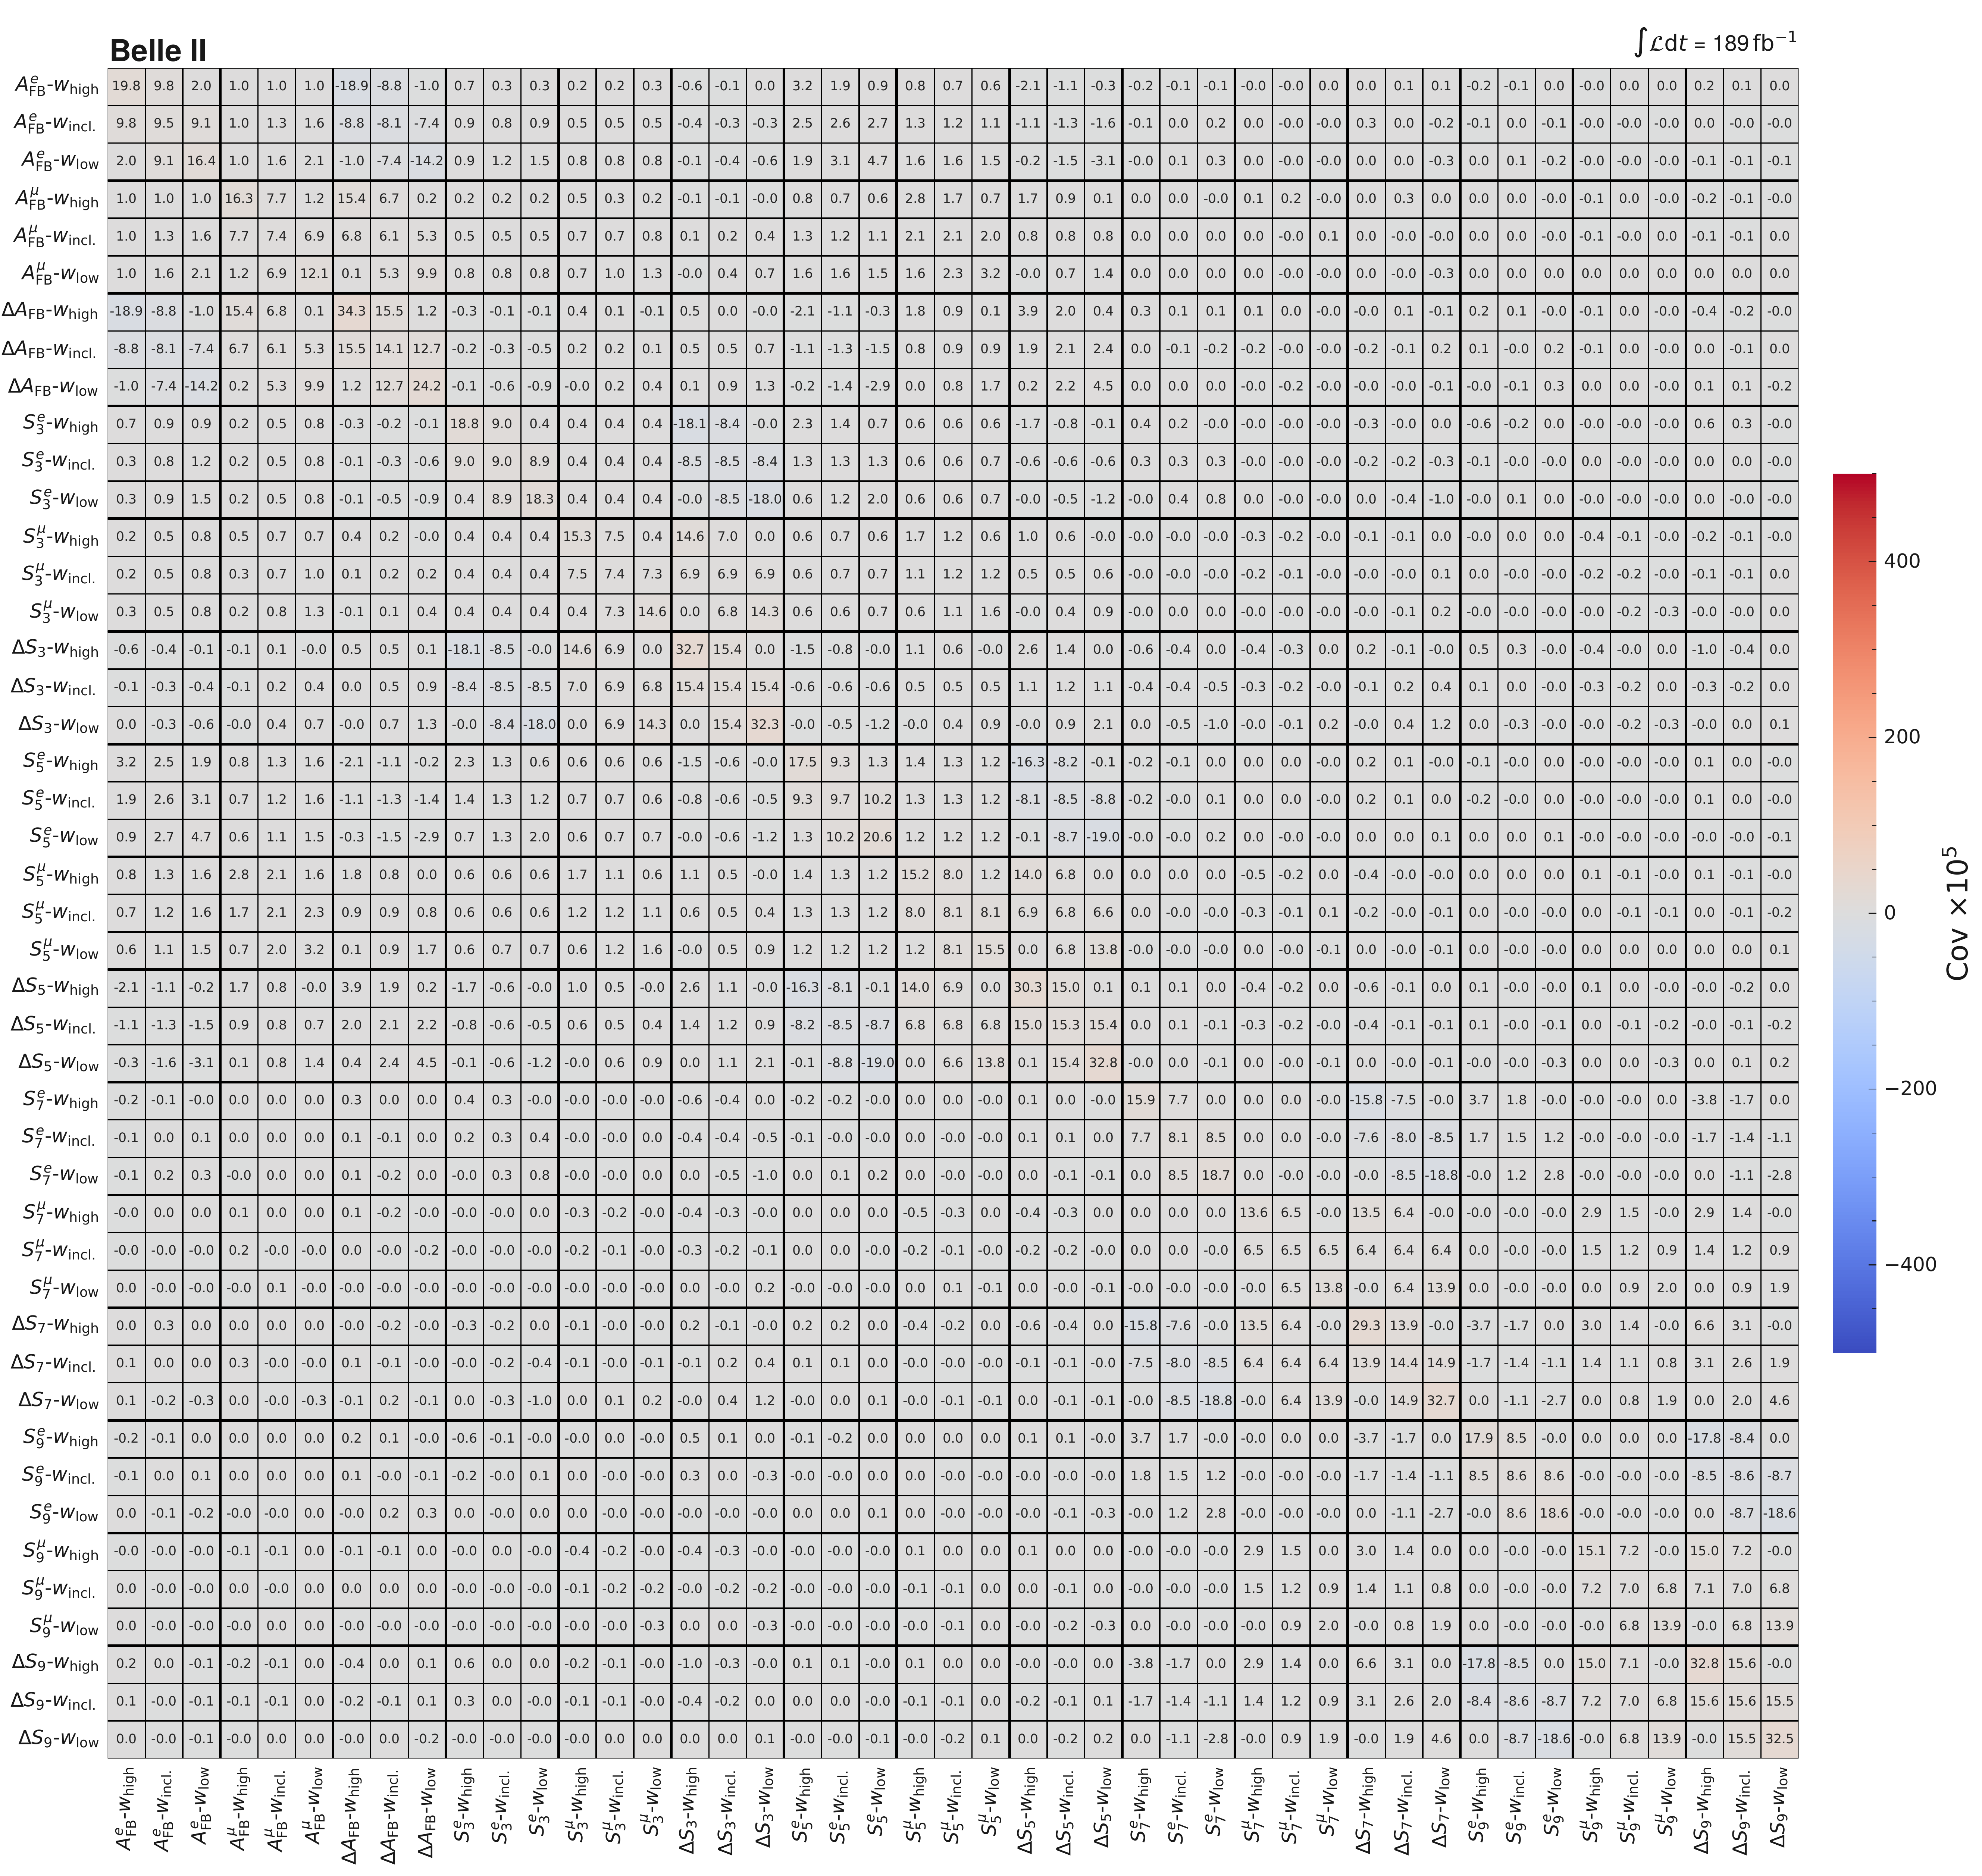}

  \caption{Systematic covariance matrix, using the same color scale as Fig.~\ref{fig:cov_stats} in order to illustrate the relative contributions to the total covariance matrix. }
  \label{fig:cov_syst}
\end{figure*}
