# Supplementary material for: Tests of light-lepton universality in angular asymmetries of $B^0 \to D^{*-} \ell \nu$ decays
Source: arXiv:2308.02023 source file (2023-11-02)
Supplement: Supplementary file 2 [file afb_results_table_sm.tex]

\begin{table}
\centering
\caption{: Full results and total uncertainties from all angular observables along with the standard model expectations.}
\label{tab:results_sm}
\begin{tabular}{llrc}
\toprule
                     Obs. &             $w$ bin &       Measurement &    SM \\
\midrule
      $A_{\mathrm{FB}}^e$ &    $w_\mathrm{low}$ &   $0.149\pm0.045$ &   $\phantom{-}0.272\pm0.005$ \\
                          &   $w_\mathrm{high}$ &   $0.213\pm0.051$ &   $\phantom{-}0.209\pm0.003$ \\
                          &  $w_\mathrm{incl.}$ &   $0.183\pm0.033$ &   $\phantom{-}0.244\pm0.004$ \\
    $A_{\mathrm{FB}}^\mu$ &    $w_\mathrm{low}$ &    $0.248\pm0.040$ &  $\phantom{-}0.271\pm0.005$ \\
                          &   $w_\mathrm{high}$ &   $0.045\pm0.051$ &   $\phantom{-}0.198\pm0.003$ \\
                          &  $w_\mathrm{incl.}$ &   $0.158\pm0.032$ &   $\phantom{-}0.239\pm0.004$ \\
 $\Delta A_{\mathrm{FB}}$ &    $w_\mathrm{low}$ &    $0.099\pm0.060$ &  $\phantom{l000000}(-1.04\pm0.02)\times 10^{-3}$ \\
                          &   $w_\mathrm{high}$ &  $-0.168\pm0.073$ &   $\phantom{l00000}(-11.33\pm0.09)\times 10^{-3}$ \\
                          &  $w_\mathrm{incl.}$ &  $-0.024\pm0.046$ &   $\phantom{l000000}(-5.66\pm0.06)\times 10^{-3}$ \\
                  $S_3^e$ &    $w_\mathrm{low}$ &  $-0.133\pm0.053$ &   $-0.147\pm0.002$ \\
                          &   $w_\mathrm{high}$ &  $-0.016\pm0.053$ &   $-0.063\pm0.002$ \\
                          &  $w_\mathrm{incl.}$ &   $-0.080\pm0.037$ &  $-0.110\pm0.002$ \\
                $S_3^\mu$ &    $w_\mathrm{low}$ &  $-0.159\pm0.048$ &   $-0.147\pm0.002$ \\
                          &   $w_\mathrm{high}$ &  $-0.117\pm0.051$ &   $-0.063\pm0.002$ \\
                          &  $w_\mathrm{incl.}$ &  $-0.142\pm0.034$ &   $-0.110\pm0.002$ \\
             $\Delta S_3$ &    $w_\mathrm{low}$ &  $-0.026\pm0.072$ &   $\phantom{00000000}(0.279\pm0.002)\times 10^{-3}$ \\
                          &   $w_\mathrm{high}$ &  $-0.101\pm0.073$ &   $\phantom{00000000}(0.233\pm0.008)\times 10^{-3}$ \\
                          &  $w_\mathrm{incl.}$ &   $-0.062\pm0.050$ &  $\phantom{00000000}(0.176\pm0.005)\times 10^{-3}$ \\
                  $S_5^e$ &    $w_\mathrm{low}$ &   $0.166\pm0.054$ &   $\phantom{-}0.172\pm0.004$ \\
                          &   $w_\mathrm{high}$ &    $0.215\pm0.050$ &  $\phantom{-}0.221\pm0.004$ \\
                          &  $w_\mathrm{incl.}$ &    $0.190\pm0.036$ &  $\phantom{-}0.194\pm0.004$ \\
                $S_5^\mu$ &    $w_\mathrm{low}$ &   $0.146\pm0.049$ &   $\phantom{-}0.172\pm0.004$ \\
                          &   $w_\mathrm{high}$ &    $0.160\pm0.048$ &  $\phantom{-}0.222\pm0.004$ \\
                          &  $w_\mathrm{incl.}$ &   $0.155\pm0.034$ &   $\phantom{-}0.194\pm0.004$ \\
             $\Delta S_5$ &    $w_\mathrm{low}$ &  $-0.019\pm0.073$ &   $\phantom{00000000}(0.272\pm0.003)\times 10^{-3}$ \\
                          &   $w_\mathrm{high}$ &  $-0.055\pm0.069$ &   $\phantom{000000000}(1.07\pm0.04)\phantom{0}\times 10^{-3}$ \\
                          &  $w_\mathrm{incl.}$ &  $-0.035\pm0.049$ &   $\phantom{000000000}(0.49\pm0.02)\phantom{0}\times 10^{-3}$ \\
                  $S_7^e$ &    $w_\mathrm{low}$ &  $-0.088\pm0.053$ &     $\phantom{l000}0.0\pm0.0\phantom{00}$ \\
                          &   $w_\mathrm{high}$ &   $0.045\pm0.049$ &           $\phantom{-}0.0\pm0.0$ \\
                          &  $w_\mathrm{incl.}$ &  $-0.018\pm0.035$ &           $\phantom{-}0.0\pm0.0$ \\
                $S_7^\mu$ &    $w_\mathrm{low}$ &   $-0.060\pm0.047$ &           $\phantom{-}0.0\pm0.0$ \\
                          &   $w_\mathrm{high}$ &   $-0.020\pm0.047$ &           $\phantom{-}0.0\pm0.0$ \\
                          &  $w_\mathrm{incl.}$ &  $-0.043\pm0.033$ &           $\phantom{-}0.0\pm0.0$ \\
             $\Delta S_7$ &    $w_\mathrm{low}$ &   $0.028\pm0.071$ &           $\phantom{-}0.0\pm0.0$ \\
                          &   $w_\mathrm{high}$ &  $-0.066\pm0.069$ &           $\phantom{-}0.0\pm0.0$ \\
                          &  $w_\mathrm{incl.}$ &  $-0.026\pm0.049$ &           $\phantom{-}0.0\pm0.0$ \\
                  $S_9^e$ &    $w_\mathrm{low}$ &  $-0.035\pm0.054$ &           $\phantom{-}0.0\pm0.0$ \\
                          &   $w_\mathrm{high}$ &    $0.020\pm0.052$ &           $\phantom{-}0.0\pm0.0$ \\
                          &  $w_\mathrm{incl.}$ &  $-0.004\pm0.036$ &           $\phantom{-}0.0\pm0.0$ \\
                $S_9^\mu$ &    $w_\mathrm{low}$ &  $-0.003\pm0.048$ &           $\phantom{-}0.0\pm0.0$ \\
                          &   $w_\mathrm{high}$ &    $0.040\pm0.050$ &           $\phantom{-}0.0\pm0.0$ \\
                          &  $w_\mathrm{incl.}$ &   $0.016\pm0.034$ &           $\phantom{-}0.0\pm0.0$ \\
             $\Delta S_9$ &    $w_\mathrm{low}$ &   $0.032\pm0.071$ &           $\phantom{-}0.0\pm0.0$ \\
                          &   $w_\mathrm{high}$ &    $0.020\pm0.072$ &           $\phantom{-}0.0\pm0.0$ \\
                          &  $w_\mathrm{incl.}$ &     $0.020\pm0.050$ &           $\phantom{-}0.0\pm0.0$ \\
\bottomrule
\end{tabular}
\end{table}
