# Supplementary material for: Tests of light-lepton universality in angular asymmetries of $B^0 \to D^{*-} \ell \nu$ decays
Source: arXiv:2308.02023 source file (2023-11-02)
Supplement: Supplementary file 3 [file afb_syst_table_sm.tex]

\begin{table}
\centering
\caption{Summary of the experimental uncertainties for all angular observables (Obs.) classified by relevant source: sample size (Stat.), MC sample size (MC stat.), lepton ID (LID), and slow-pion efficiency ($\pi_{	\textrm{slow}}$).}
\label{tab:systematics_sm}
\begin{tabular}{llccccc}
\toprule
                     Obs. &             $w$ bin &  Total &  Stat. &  MC stat. &    LID &  $\pi_{\textrm{slow}}$ \\
\midrule
      $A_{\mathrm{FB}}^e$ &    $w_\mathrm{low}$ &  0.045 &  0.042 &     0.015 &  0.004 &                  0.001 \\
                          &   $w_\mathrm{high}$ &  0.051 &  0.048 &     0.017 &  0.004 &                  0.001 \\
                          &  $w_\mathrm{incl.}$ &  0.033 &  0.031 &     0.011 &  0.004 &                  0.001 \\
    $A_{\mathrm{FB}}^\mu$ &    $w_\mathrm{low}$ &  0.040 &  0.038 &     0.013 &  0.001 &                  0.001 \\
                          &   $w_\mathrm{high}$ &  0.051 &  0.048 &     0.016 &  0.002 &                  0.001 \\
                          &  $w_\mathrm{incl.}$ &  0.032 &  0.030 &     0.010 &  0.001 &                  0.001 \\
 $\Delta A_{\mathrm{FB}}$ &    $w_\mathrm{low}$ &  0.060 &  0.056 &     0.020 &  0.004 &                  0.001 \\
                          &   $w_\mathrm{high}$ &  0.073 &  0.068 &     0.024 &  0.004 &                  0.001 \\
                          &  $w_\mathrm{incl.}$ &  0.046 &  0.043 &     0.015 &  0.004 &                  0.001 \\
                  $S_3^e$ &    $w_\mathrm{low}$ &  0.053 &  0.050 &     0.018 &  $<0.001\phantom{0~~}$ &                  0.001 \\
                          &   $w_\mathrm{high}$ &  0.053 &  0.049 &     0.018 &  $<0.001\phantom{0~~}$ &                  $<0.001\phantom{0~~}$ \\
                          &  $w_\mathrm{incl.}$ &  0.037 &  0.034 &     0.012 &  $<0.001\phantom{0~~}$ &                  $<0.001\phantom{0~~}$ \\
                $S_3^\mu$ &    $w_\mathrm{low}$ &  0.048 &  0.045 &     0.016 &  0.001 &                  $<0.001\phantom{0~~}$ \\
                          &   $w_\mathrm{high}$ &  0.051 &  0.048 &     0.016 &  $<0.001\phantom{0~~}$ &                  $<0.001\phantom{0~~}$ \\
                          &  $w_\mathrm{incl.}$ &  0.034 &  0.032 &     0.011 &  0.001 &                  $<0.001\phantom{0~~}$ \\
             $\Delta S_3$ &    $w_\mathrm{low}$ &  0.072 &  0.068 &     0.024 &  0.001 &                  $<0.001\phantom{0~~}$ \\
                          &   $w_\mathrm{high}$ &  0.073 &  0.069 &     0.025 &  0.001 &                  $<0.001\phantom{0~~}$ \\
                          &  $w_\mathrm{incl.}$ &  0.050 &  0.047 &     0.017 &  0.001 &                  $<0.001\phantom{0~~}$ \\
                  $S_5^e$ &    $w_\mathrm{low}$ &  0.054 &  0.051 &     0.018 &  0.001 &                  $<0.001\phantom{0~~}$ \\
                          &   $w_\mathrm{high}$ &  0.050 &  0.047 &     0.017 &  0.001 &                  $<0.001\phantom{0~~}$ \\
                          &  $w_\mathrm{incl.}$ &  0.036 &  0.034 &     0.012 &  0.001 &                  $<0.001\phantom{0~~}$ \\
                $S_5^\mu$ &    $w_\mathrm{low}$ &  0.049 &  0.046 &     0.016 &  0.001 &                  $<0.001\phantom{0~~}$ \\
                          &   $w_\mathrm{high}$ &  0.048 &  0.045 &     0.016 &  $<0.001\phantom{0~~}$ &                  $<0.001\phantom{0~~}$ \\
                          &  $w_\mathrm{incl.}$ &  0.034 &  0.032 &     0.011 &  $<0.001\phantom{0~~}$ &                  $<0.001\phantom{0~~}$ \\
             $\Delta S_5$ &    $w_\mathrm{low}$ &  0.073 &  0.068 &     0.024 &  0.001 &                  $<0.001\phantom{0~~}$ \\
                          &   $w_\mathrm{high}$ &  0.069 &  0.065 &     0.023 &  0.001 &                  $<0.001\phantom{0~~}$ \\
                          &  $w_\mathrm{incl.}$ &  0.049 &  0.046 &     0.016 &  0.001 &                  $<0.001\phantom{0~~}$ \\
                  $S_7^e$ &    $w_\mathrm{low}$ &  0.053 &  0.050 &     0.018 &  0.001 &                  $<0.001\phantom{0~~}$ \\
                          &   $w_\mathrm{high}$ &  0.049 &  0.046 &     0.017 &  $<0.001\phantom{0~~}$ &                  $<0.001\phantom{0~~}$ \\
                          &  $w_\mathrm{incl.}$ &  0.035 &  0.033 &     0.012 &  $<0.001\phantom{0~~}$ &                  $<0.001\phantom{0~~}$ \\
                $S_7^\mu$ &    $w_\mathrm{low}$ &  0.047 &  0.045 &     0.015 &  $<0.001\phantom{0~~}$ &                  $<0.001\phantom{0~~}$ \\
                          &   $w_\mathrm{high}$ &  0.047 &  0.045 &     0.015 &  $<0.001\phantom{0~~}$ &                  $<0.001\phantom{0~~}$ \\
                          &  $w_\mathrm{incl.}$ &  0.033 &  0.031 &     0.011 &  $<0.001\phantom{0~~}$ &                  $<0.001\phantom{0~~}$ \\
             $\Delta S_7$ &    $w_\mathrm{low}$ &  0.071 &  0.067 &     0.023 &  0.001 &                  0.001 \\
                          &   $w_\mathrm{high}$ &  0.069 &  0.065 &     0.022 &  $<0.001\phantom{0~~}$ &                  $<0.001\phantom{0~~}$ \\
                          &  $w_\mathrm{incl.}$ &  0.049 &  0.046 &     0.016 &  $<0.001\phantom{0~~}$ &                  $<0.001\phantom{0~~}$ \\
                  $S_9^e$ &    $w_\mathrm{low}$ &  0.054 &  0.050 &     0.018 &  $<0.001\phantom{0~~}$ &                  $<0.001\phantom{0~~}$ \\
                          &   $w_\mathrm{high}$ &  0.052 &  0.049 &     0.018 &  $<0.001\phantom{0~~}$ &                  $<0.001\phantom{0~~}$ \\
                          &  $w_\mathrm{incl.}$ &  0.036 &  0.034 &     0.012 &  $<0.001\phantom{0~~}$ &                  $<0.001\phantom{0~~}$ \\
                $S_9^\mu$ &    $w_\mathrm{low}$ &  0.048 &  0.046 &     0.016 &  $<0.001\phantom{0~~}$ &                  $<0.001\phantom{0~~}$ \\
                          &   $w_\mathrm{high}$ &  0.050 &  0.047 &     0.016 &  $<0.001\phantom{0~~}$ &                  0.001 \\
                          &  $w_\mathrm{incl.}$ &  0.034 &  0.032 &     0.011 &  $<0.001\phantom{0~~}$ &                  $<0.001\phantom{0~~}$ \\
             $\Delta S_9$ &    $w_\mathrm{low}$ &  0.071 &  0.067 &     0.024 &  $<0.001\phantom{0~~}$ &                  $<0.001\phantom{0~~}$ \\
                          &   $w_\mathrm{high}$ &  0.072 &  0.068 &     0.024 &  0.001 &                  0.001 \\
                          &  $w_\mathrm{incl.}$ &  0.050 &  0.047 &     0.017 &  $<0.001\phantom{0~~}$ &                  $<0.001\phantom{0~~}$ \\
\bottomrule
\end{tabular}
\end{table}
