# Supplementary material for: Tests of light-lepton universality in angular asymmetries of $B^0 \to D^{*-} \ell \nu$ decays
Source: arXiv:2308.02023 source file (2023-11-02)
Supplement: Supplementary file 4 [file afb_results_table_sm_BACKUP.tex]

\begin{table}
\centering
\caption{: Full results and total uncertainties from all angular observables (Obs.) along with the standard model expectations (SM).}
\label{tab:results_sm}
\begin{tabular}{llrr}
\toprule
                     Obs. &             $w$ bin &       Measurement &       SM$\phantom{000000}$ \\
\midrule
      $A_{\mathrm{FB}}^e$ &    $w_\mathrm{low}$ &   $0.149\pm0.045$ &   $0.27212\pm0.00456$ \\
                          &   $w_\mathrm{high}$ &   $0.213\pm0.051$ &   $0.20939\pm0.00295$ \\
                          &  $w_\mathrm{incl.}$ &   $0.183\pm0.033$ &   $0.24440\pm0.00366$ \\
    $A_{\mathrm{FB}}^\mu$ &    $w_\mathrm{low}$ &    $0.248\pm0.040$ &  $0.27108\pm0.00454$ \\
                          &   $w_\mathrm{high}$ &   $0.045\pm0.051$ &   $0.19806\pm0.00296$ \\
                          &  $w_\mathrm{incl.}$ &   $0.158\pm0.032$ &   $0.23874\pm0.00365$ \\
 $\Delta A_{\mathrm{FB}}$ &    $w_\mathrm{low}$ &    $0.099\pm0.060$ &  $-0.00104\pm0.00002$ \\
                          &   $w_\mathrm{high}$ &  $-0.168\pm0.073$ &   $-0.01133\pm0.00009$ \\
                          &  $w_\mathrm{incl.}$ &  $-0.024\pm0.046$ &   $-0.00566\pm0.00006$ \\
                  $S_3^e$ &    $w_\mathrm{low}$ &  $-0.133\pm0.053$ &   $-0.14701\pm0.00190$ \\
                          &   $w_\mathrm{high}$ &  $-0.016\pm0.053$ &   $-0.06280\pm0.00200$ \\
                          &  $w_\mathrm{incl.}$ &   $-0.080\pm0.037$ &  $-0.10980\pm0.00198$ \\
                $S_3^\mu$ &    $w_\mathrm{low}$ &  $-0.159\pm0.048$ &   $-0.14673\pm0.00190$ \\
                          &   $w_\mathrm{high}$ &  $-0.117\pm0.051$ &   $-0.06257\pm0.00200$ \\
                          &  $w_\mathrm{incl.}$ &  $-0.142\pm0.034$ &   $-0.10963\pm0.00198$ \\
             $\Delta S_3$ &    $w_\mathrm{low}$ &  $-0.026\pm0.072$ &   $0.00028\pm0.00000$ \\
                          &   $w_\mathrm{high}$ &  $-0.101\pm0.073$ &   $0.00023\pm0.00004$ \\
                          &  $w_\mathrm{incl.}$ &   $-0.062\pm0.050$ &  $0.00018\pm0.00001$ \\
                  $S_5^e$ &    $w_\mathrm{low}$ &   $0.166\pm0.054$ &   $0.17208\pm0.00351$ \\
                          &   $w_\mathrm{high}$ &    $0.215\pm0.050$ &  $0.22067\pm0.00373$ \\
                          &  $w_\mathrm{incl.}$ &    $0.190\pm0.036$ &  $0.19355\pm0.00356$ \\
                $S_5^\mu$ &    $w_\mathrm{low}$ &   $0.146\pm0.049$ &   $0.17235\pm0.00351$ \\
                          &   $w_\mathrm{high}$ &    $0.160\pm0.048$ &  $0.22174\pm0.00369$ \\
                          &  $w_\mathrm{incl.}$ &   $0.155\pm0.034$ &   $0.19405\pm0.00354$ \\
             $\Delta S_5$ &    $w_\mathrm{low}$ &  $-0.019\pm0.073$ &     $0.00027\pm0.00000$ \\
                          &   $w_\mathrm{high}$ &  $-0.055\pm0.069$ &     $0.00107\pm0.00004$ \\
                          &  $w_\mathrm{incl.}$ &  $-0.035\pm0.049$ &     $0.00049\pm0.00002$ \\
                  $S_7^e$ &    $w_\mathrm{low}$ &  $-0.088\pm0.053$ &     $0.0\pm0.0\phantom{0000}$ \\
                          &   $w_\mathrm{high}$ &   $0.045\pm0.049$ &           $0.0\pm0.0\phantom{0000}$ \\
                          &  $w_\mathrm{incl.}$ &  $-0.018\pm0.035$ &           $0.0\pm0.0\phantom{0000}$ \\
                $S_7^\mu$ &    $w_\mathrm{low}$ &   $-0.060\pm0.047$ &           $0.0\pm0.0\phantom{0000}$ \\
                          &   $w_\mathrm{high}$ &   $-0.020\pm0.047$ &           $0.0\pm0.0\phantom{0000}$ \\
                          &  $w_\mathrm{incl.}$ &  $-0.043\pm0.033$ &           $0.0\pm0.0\phantom{0000}$ \\
             $\Delta S_7$ &    $w_\mathrm{low}$ &   $0.028\pm0.071$ &           $0.0\pm0.0\phantom{0000}$ \\
                          &   $w_\mathrm{high}$ &  $-0.066\pm0.069$ &           $0.0\pm0.0\phantom{0000}$ \\
                          &  $w_\mathrm{incl.}$ &  $-0.026\pm0.049$ &           $0.0\pm0.0\phantom{0000}$ \\
                  $S_9^e$ &    $w_\mathrm{low}$ &  $-0.035\pm0.054$ &           $0.0\pm0.0\phantom{0000}$ \\
                          &   $w_\mathrm{high}$ &    $0.020\pm0.052$ &           $0.0\pm0.0\phantom{0000}$ \\
                          &  $w_\mathrm{incl.}$ &  $-0.004\pm0.036$ &           $0.0\pm0.0\phantom{0000}$ \\
                $S_9^\mu$ &    $w_\mathrm{low}$ &  $-0.003\pm0.048$ &           $0.0\pm0.0\phantom{0000}$ \\
                          &   $w_\mathrm{high}$ &    $0.040\pm0.050$ &           $0.0\pm0.0\phantom{0000}$ \\
                          &  $w_\mathrm{incl.}$ &   $0.016\pm0.034$ &           $0.0\pm0.0\phantom{0000}$ \\
             $\Delta S_9$ &    $w_\mathrm{low}$ &   $0.032\pm0.071$ &           $0.0\pm0.0\phantom{0000}$ \\
                          &   $w_\mathrm{high}$ &    $0.020\pm0.072$ &           $0.0\pm0.0\phantom{0000}$ \\
                          &  $w_\mathrm{incl.}$ &     $0.020\pm0.050$ &           $0.0\pm0.0\phantom{0000}$ \\
\bottomrule
\end{tabular}
\end{table}
