# Supplementary material for: Tests of light-lepton universality in angular asymmetries of $B^0 \to D^{*-} \ell \nu$ decays
Source: arXiv:2308.02023 source file (2023-11-02)
Supplement: Supplementary file 5 [file afb_results_table_sm_OLD.tex]

\begin{table}[]
  \centering
  \caption{Full results from all angular observables (Obs.) along with the standard model expectations (SM).}
  \label{tab:results_sm}
  \sisetup{
    separate-uncertainty=true, % controls whether uncertainty is given by \pm or in parantheses
    table-alignment-mode=marker, % align on decimal marker
    table-align-uncertainty=true,
    table-align-exponent=true,
    bracket-ambiguous-numbers=false, % if true, adds parentheses around separate uncertainties with exponent, breaks formatting
  }
  \begin{tabular}{ll
      % siunivvvvvvvtx column types for processing uncertainties, exponents with alignment
      % HACK: I use zero-decimal-to-integer=true and 0.0 float uncertainties, because with integer 0 uncertainties siunitx drops them
      S[table-format=+1.3+-1.3]
      % in the format I set the uncertainty digits to 5 instead of 3 in order to increase the distance of the exponent in order to reduce ambiguouity with `bracket-ambiguous-numbers=false`
      S[table-format=+2.3(1.5)e+1]
    }
    \toprule
    Obs.                     & $w$ bin            & \text{Measurement} & \text{SM}      \\
    \midrule

    $A_{\mathrm{FB}}^e$      & $w_\mathrm{low}$   & 0.192+-0.045       & 0.272(0.004)  \\
                             & $w_\mathrm{high}$  & 0.228+-0.049       & 0.209(0.003)  \\
                             & $w_\mathrm{incl.}$ & 0.211+-0.03        & 0.244(0.004)  \\
    $A_{\mathrm{FB}}^\mu$    & $w_\mathrm{low}$   & 0.236+-0.042       & 0.271(0.005)  \\
                             & $w_\mathrm{high}$  & 0.068+-0.047       & 0.198(0.003)  \\
                             & $w_\mathrm{incl.}$ & 0.16+-0.031        & 0.239(0.004)  \\
    $\Delta A_{\mathrm{FB}}$ & $w_\mathrm{low}$   & 0.044+-0.061       & -1.04(0.02)e-3     \\
                             & $w_\mathrm{high}$  & -0.16+-0.068       & -11.33(0.09)e-3    \\
                             & $w_\mathrm{incl.}$ & -0.051+-0.043      & -5.66(0.06)e-3     \\
    $S_3^e$                  & $w_\mathrm{low}$   & -0.156+-0.048      & -0.147(0.002) \\
                             & $w_\mathrm{high}$  & -0.004+-0.048      & -0.063(.002)  \\
                             & $w_\mathrm{incl.}$ & -0.087+-0.032      & -0.110(.002) \\
    $S_3^\mu$                & $w_\mathrm{low}$   & -0.17+-0.046       & -0.147(0.002) \\
                             & $w_\mathrm{high}$  & -0.138+-0.048      & -0.063(0.002)  \\
                             & $w_\mathrm{incl.}$ & -0.159+-0.033      & -0.111(0.002) \\
    $\Delta S_3$             & $w_\mathrm{low}$   & -0.014+-0.067      & 2.79(0.02)e-4  \\
                             & $w_\mathrm{high}$  & -0.134+-0.068      & 2.33(0.08)e-4    \\
                             & $w_\mathrm{incl.}$ & -0.072+-0.046      & 1.76(0.06)e-4    \\
    $S_5^e$                  & $w_\mathrm{low}$   & 0.152+-0.05        & 0.172(0.004)  \\
                             & $w_\mathrm{high}$  & 0.225+-0.048       & 0.221(0.004)  \\
                             & $w_\mathrm{incl.}$ & 0.187+-0.035       & 0.194(0.004)  \\
    $S_5^\mu$                & $w_\mathrm{low}$   & 0.156+-0.046       & 0.172(0.004)  \\
                             & $w_\mathrm{high}$  & 0.162+-0.047       & 0.222(0.004)  \\
                             & $w_\mathrm{incl.}$ & 0.159+-0.031       & 0.194(0.004)  \\
    $\Delta S_5$             & $w_\mathrm{low}$   & 0.004+-0.068       & 2.72(0.03)e-4  \\
                             & $w_\mathrm{high}$  & -0.063+-0.067      & 10.7(0.4)e-4   \\
                             & $w_\mathrm{incl.}$ & -0.028+-0.047      & 4.93(0.21)e-4    \\
    $S_7^e$                  & $w_\mathrm{low}$   & -0.082+-0.048      & 0(0)      \\
                             & $w_\mathrm{high}$  & 0.026+-0.046       & 0(0)      \\
                             & $w_\mathrm{incl.}$ & -0.024+-0.032      & 0(0)      \\
    $S_7^\mu$                & $w_\mathrm{low}$   & -0.083+-0.045      & 0(0)      \\
                             & $w_\mathrm{high}$  & -0.033+-0.046      & 0(0)      \\
                             & $w_\mathrm{incl.}$ & -0.06+-0.031       & 0(0)      \\
    $\Delta S_7$             & $w_\mathrm{low}$   & -0.001+-0.066      & 0(0)      \\
                             & $w_\mathrm{high}$  & -0.06+-0.065       & 0(0)      \\
                             & $w_\mathrm{incl.}$ & -0.036+-0.044      & 0(0)      \\
    $S_9^e$                  & $w_\mathrm{low}$   & -0.026+-0.049      & 0(0)      \\
                             & $w_\mathrm{high}$  & 0.01+-0.048        & 0(0)      \\
                             & $w_\mathrm{incl.}$ & -0.005+-0.034      & 0(0)      \\
    $S_9^\mu$                & $w_\mathrm{low}$   & -0.023+-0.045      & 0(0)      \\
                             & $w_\mathrm{high}$  & 0.046+-0.047       & 0(0)      \\
                             & $w_\mathrm{incl.}$ & 0.01+-0.032        & 0(0)      \\
    $\Delta S_9$             & $w_\mathrm{low}$   & 0.003+-0.067       & 0(0)      \\
                             & $w_\mathrm{high}$  & 0.036+-0.067       & 0(0)      \\
                             & $w_\mathrm{incl.}$ & 0.015+-0.046       & 0(0)      \\
    \bottomrule
  \end{tabular}
\end{table}
