# Supplementary material for: Tests of light-lepton universality in angular asymmetries of $B^0 \to D^{*-} \ell \nu$ decays
Source: arXiv:2308.02023 source file (2023-11-02)
Supplement: Supplementary file 6 [file afb_syst_table_sm_OLD.tex]

\begin{table}
  \centering
  \caption{A breakdown of the experimental uncertainties for all angular observables (Obs.) by relevant source: sample size (Stat.), MC sample size (MC stat.), lepton ID (LID), and slow pion efficiency ($\pi_{\textrm{slow}}$).}
  \label{tab:systematics_sm}
  \sisetup{table-format=1.3}
  \begin{tabular}{llSSSSS}
    \toprule
    Obs.                     & $w$ bin            & \text{Total} & \text{Stat.} & \text{MC stat.} & \text{LID} & $\pi_{\textrm{slow}}$ \\
    \midrule
    $A_{\mathrm{FB}}^e$      & $w_\mathrm{low}$  & 
     0.049 &  0.047 &     0.013 &  0.004 &                  0.001 \\
                           &   $w_\mathrm{high}$ &  0.049 &  0.047 &     0.013 &  0.004 &                  0.001 \\    
                          &  $w_\mathrm{incl.}$ &  0.031 &  0.029 &     0.008 &  0.003 &                  0.001 \\
    $A_{\mathrm{FB}}^\mu$ &    $w_\mathrm{low}$ &  0.042 &  0.041 &     0.010 &  0.001 &                  0.000 \\
                          &   $w_\mathrm{high}$ &  0.048 &  0.046 &     0.012 &  0.002 &                  0.001 \\
                          &  $w_\mathrm{incl.}$ &  0.031 &  0.030 &     0.008 &  0.001 &                  0.001 \\
 $\Delta A_{\mathrm{FB}}$ &    $w_\mathrm{low}$ &  0.062 &  0.060 &     0.015 &  0.004 &                  0.001 \\
                          &   $w_\mathrm{high}$ &  0.068 &  0.066 &     0.018 &  0.004 &                  0.000 \\
                          &  $w_\mathrm{incl.}$ &  0.043 &  0.042 &     0.011 &  0.004 &                  0.001 \\
                  $S_3^e$ &    $w_\mathrm{low}$ &  0.048 &  0.046 &     0.013 &  0.000 &                  0.001 \\
                          &   $w_\mathrm{high}$ &  0.049 &  0.047 &     0.014 &  0.000 &                  0.000 \\
                          &  $w_\mathrm{incl.}$ &  0.033 &  0.031 &     0.009 &  0.000 &                  0.000 \\
                $S_3^\mu$ &    $w_\mathrm{low}$ &  0.046 &  0.045 &     0.012 &  0.000 &                  0.000 \\
                          &   $w_\mathrm{high}$ &  0.048 &  0.046 &     0.012 &  0.000 &                  0.000 \\
                          &  $w_\mathrm{incl.}$ &  0.033 &  0.032 &     0.008 &  0.000 &                  0.000 \\
             $\Delta S_3$ &    $w_\mathrm{low}$ &  0.067 &  0.065 &     0.018 &  0.001 &                  0.001 \\
                          &   $w_\mathrm{high}$ &  0.068 &  0.066 &     0.018 &  0.001 &                  0.000 \\
                          &  $w_\mathrm{incl.}$ &  0.046 &  0.044 &     0.012 &  0.001 &                  0.000 \\
                  $S_5^e$ &    $w_\mathrm{low}$ &  0.051 &  0.049 &     0.014 &  0.001 &                  0.001 \\
                          &   $w_\mathrm{high}$ &  0.048 &  0.047 &     0.013 &  0.001 &                  0.000 \\
                          &  $w_\mathrm{incl.}$ &  0.035 &  0.034 &     0.009 &  0.001 &                  0.000 \\
                $S_5^\mu$ &    $w_\mathrm{low}$ &  0.046 &  0.045 &     0.012 &  0.000 &                  0.000 \\
                          &   $w_\mathrm{high}$ &  0.047 &  0.045 &     0.012 &  0.000 &                  0.000 \\
                          &  $w_\mathrm{incl.}$ &  0.031 &  0.030 &     0.008 &  0.000 &                  0.000 \\
             $\Delta S_5$ &    $w_\mathrm{low}$ &  0.069 &  0.066 &     0.018 &  0.001 &                  0.001 \\
                          &   $w_\mathrm{high}$ &  0.067 &  0.065 &     0.017 &  0.001 &                  0.000 \\
                          &  $w_\mathrm{incl.}$ &  0.047 &  0.045 &     0.012 &  0.001 &                  0.000 \\
                  $S_7^e$ &    $w_\mathrm{low}$ &  0.048 &  0.046 &     0.014 &  0.000 &                  0.000 \\
                          &   $w_\mathrm{high}$ &  0.047 &  0.045 &     0.013 &  0.000 &                  0.000 \\
                          &  $w_\mathrm{incl.}$ &  0.032 &  0.030 &     0.009 &  0.000 &                  0.000 \\
                $S_7^\mu$ &    $w_\mathrm{low}$ &  0.045 &  0.044 &     0.012 &  0.000 &                  0.000 \\
                          &   $w_\mathrm{high}$ &  0.046 &  0.044 &     0.012 &  0.000 &                  0.000 \\
                          &  $w_\mathrm{incl.}$ &  0.031 &  0.030 &     0.008 &  0.000 &                  0.000 \\
             $\Delta S_7$ &    $w_\mathrm{low}$ &  0.066 &  0.063 &     0.018 &  0.000 &                  0.000 \\
                          &   $w_\mathrm{high}$ &  0.066 &  0.063 &     0.017 &  0.000 &                  0.000 \\
                          &  $w_\mathrm{incl.}$ &  0.045 &  0.043 &     0.012 &  0.000 &                  0.000 \\
                  $S_9^e$ &    $w_\mathrm{low}$ &  0.050 &  0.048 &     0.014 &  0.000 &                  0.000 \\
                          &   $w_\mathrm{high}$ &  0.049 &  0.047 &     0.013 &  0.000 &                  0.000 \\
                          &  $w_\mathrm{incl.}$ &  0.034 &  0.033 &     0.009 &  0.000 &                  0.000 \\
                $S_9^\mu$ &    $w_\mathrm{low}$ &  0.045 &  0.044 &     0.012 &  0.000 &                  0.000 \\
                          &   $w_\mathrm{high}$ &  0.048 &  0.046 &     0.012 &  0.000 &                  0.000 \\
                          &  $w_\mathrm{incl.}$ &  0.032 &  0.031 &     0.008 &  0.000 &                  0.000 \\
             $\Delta S_9$ &    $w_\mathrm{low}$ &  0.067 &  0.065 &     0.018 &  0.000 &                  0.000 \\
                          &   $w_\mathrm{high}$ &  0.068 &  0.065 &     0.018 &  0.000 &                  0.000 \\
                          &  $w_\mathrm{incl.}$ &  0.047 &  0.045 &     0.012 &  0.000 &                  0.000 \\
    \bottomrule
  \end{tabular}
\end{table}
